# Supplementary material for: Learning Optimal Solutions via an LSTM-Optimization Framework
Source: arXiv:2207.02937 source file (2022-07-06)
Supplement: Supplementary file 2 [file zzAppendicesAUXfile.tex]

\begin{filecontents}{zzAppendices.aux}
\relax 
\providecommand\hyper@newdestlabel[2]{}
\providecommand\HyperFirstAtBeginDocument{\AtBeginDocument}
\HyperFirstAtBeginDocument{\ifx\hyper@anchor\@undefined
	\global\let\oldcontentsline\contentsline
	\gdef\contentsline#1#2#3#4{\oldcontentsline{#1}{#2}{#3}}
	\global\let\oldnewlabel\newlabel
	\gdef\newlabel#1#2{\newlabelxx{#1}#2}
	\gdef\newlabelxx#1#2#3#4#5#6{\oldnewlabel{#1}{{#2}{#3}}}
	\AtEndDocument{\ifx\hyper@anchor\@undefined
		\let\contentsline\oldcontentsline
		\let\newlabel\oldnewlabel
		\fi}
	\fi}
\global\let\hyper@last\relax 
\gdef\HyperFirstAtBeginDocument#1{#1}
\providecommand\HyField@AuxAddToFields[1]{}
\providecommand\HyField@AuxAddToCoFields[2]{}
\bibstyle{chicago}
\@writefile{toc}{\contentsline {section}{\numberline {A1}Results for Training LSTM Models}{1}{section.1}\protected@file@percent }
\newlabel{Results for Training LSTM Models}{{A1}{1}{Results for Training LSTM Models}{section.1}{}}
\@writefile{lot}{\contentsline {table}{\numberline {A1}{\ignorespaces LSTM training times for the model with the highest validation accuracy (in CPU seconds)}}{1}{table.1}\protected@file@percent }
\newlabel{traintimes}{{A1}{1}{LSTM training times for the model with the highest validation accuracy (in CPU seconds)}{table.1}{}}
\@writefile{toc}{\contentsline {section}{\numberline {A2}More Results on the Experiments}{2}{section.2}\protected@file@percent }
\newlabel{More Results on the Experiments}{{A2}{2}{More Results on the Experiments}{section.2}{}}
\@writefile{lot}{\contentsline {table}{\numberline {A2}{\ignorespaces Summary of experiments for $f = 1,000$ and $T = 90$}}{3}{table.2}\protected@file@percent }
\newlabel{t:f1,000t90}{{A2}{3}{Summary of experiments for $f = 1,000$ and $T = 90$}{table.2}{}}
\@writefile{lot}{\contentsline {table}{\numberline {A3}{\ignorespaces Summary of experiments for $f = 10,000$ and $T = 90$}}{4}{table.3}\protected@file@percent }
\newlabel{t:f10,000t90}{{A3}{4}{Summary of experiments for $f = 10,000$ and $T = 90$}{table.3}{}}
\@writefile{toc}{\contentsline {section}{\numberline {A3}Predicting Instances with Different Distributions}{4}{section.3}\protected@file@percent }
\newlabel{Predicting Instances with Different Distributions}{{A3}{4}{Predicting Instances with Different Distributions}{section.3}{}}
\@writefile{lot}{\contentsline {table}{\numberline {A4}{\ignorespaces Summary of experiments for $f = 1,000$ and $T = 120$}}{5}{table.4}\protected@file@percent }
\newlabel{t:f1,000t120}{{A4}{5}{Summary of experiments for $f = 1,000$ and $T = 120$}{table.4}{}}
\@writefile{lot}{\contentsline {table}{\numberline {A5}{\ignorespaces Summary of generalization experiments to test datasets with different characteristics}}{7}{table.5}\protected@file@percent }
\newlabel{gen1}{{A5}{7}{Summary of generalization experiments to test datasets with different characteristics}{table.5}{}}

\end{filecontents}
