# Supplementary material for: Learning Optimal Solutions via an LSTM-Optimization Framework
Source: arXiv:2207.02937 source file (2022-07-06)
Supplement: Supplementary file 3 [file zzAppendices.tex]

\documentclass[11 pt]{article}
\usepackage{latexsym}
\usepackage[tbtags]{amsmath}
\usepackage{amssymb}
\usepackage{amsmath}
%\usepackage[ruled,lined]{algorithm2e}
\usepackage{color}
\usepackage{graphicx}
\usepackage{authblk}
\usepackage{cite}
\usepackage[usenames,dvipsnames]{xcolor}
\usepackage[pdfborder={0 0 0}]{hyperref}% For email addresses
\usepackage{algorithm} 
\usepackage{algorithmic}
\usepackage{lipsum}
\usepackage{tablefootnote}
\usepackage{fixltx2e}

\newcommand\Tau{\mathcal{T}}% Caligraphic T for example

\DeclareRobustCommand{\bbone}{\text{\usefont{U}{bbold}{m}{n}1}}

\DeclareMathOperator{\EX}{\mathbb{E}}% expected value

\usepackage{hyperref}
\hypersetup{
	colorlinks=true,
	linkcolor=blue,
	filecolor=magenta,      
	urlcolor=cyan,
}

\urlstyle{same}
%\usepackage{algpseudocode}
\allowdisplaybreaks
\setlength{\oddsidemargin}{-0.1in}
%\setlength{\evensidemargin}{-0.1in}
%\setlength{\columnsep}{.2in}
\setlength{\textwidth}{6.5in}
\setlength{\topmargin}{-.5in}
\setlength{\textheight}{8.5in}
%\setlength{\parskip}{8pt}
%\setlength{\parindent}{1.0em}
%\lineskip 1pt \normallineskip 1pt
\def\baselinestretch{1.5}

\def\inclde-picture #1 by #2 (#3){%
	\vbox to #2{%
		\hrule width #1 height 0pt depth 0pt
		\vfill
		\special{picture #3}}}
\def\scaledpicture #1 by #2 (#3 scaled #4){{%
		\dimen0=#1 \dimen1=#2
		\divide\dimen0 by 1000 \multiply \dimen0 by #4
		\divide\dimen1 by 1000 \multiply \dimen1 by #4
		\inclde-picture \dimen0 by \dimen1 (#3 scaled #4)}}

%
%-----------------------Functions needed to include figures-------
%
\def\inclde-picture #1 by #2 (#3){%
	\vbox to #2{%
		\hrule width #1 height 0pt depth 0pt
		\vfill
		\special{picture #3}}}
\def\scaledpicture #1 by #2 (#3 scaled #4){{%
		\dimen0=#1 \dimen1=#2
		\divide\dimen0 by 1000 \multiply \dimen0 by #4
		\divide\dimen1 by 1000 \multiply \dimen1 by #4
		\inclde-picture \dimen0 by \dimen1 (#3 scaled #4)}}
%-------------------------- Examples---------------------------
%
\newcounter{example}
\newenvironment{example}[1]{\vspace{-.125in} 
	\refstepcounter{example}\noindent\paragraph{\bf Example 
		\arabic{example}:  \newline }}{$\Box$ \\ \vspace{-.2in}}

%\newtheorem{example}{Example}
%\newenvironment{contexample}{
%  \addtocounter{example}{-1} \begin{example}[continued]}{
% \end{example}}

%   \newcounter{example}
%\newenvironment{example}{%
%\refstepcounter{example}%
%{\bfseries Example \theexample}}{}

\newenvironment{examplecont}{%
	{\bfseries Example \theexample} (continued)}{}

\newenvironment{proof}{ {\bf Proof.}}{$\Box$ \\}
\newcounter{para}
\newenvironment{para}  {\stepcounter{para}{\bf \S\thepara}}{\\}  
%\@.\theexample
%----------------------Theorems, Lemmata and Corollaries, etc--
%
\newtheorem{theorem}{Theorem}
\newtheorem{lemma}{Lemma}
\newtheorem{claim}{Claim}
\newtheorem{corollary}{Corollary}[theorem]
\newtheorem{conjecture}{Conjecture}[section]
\newtheorem{definition}{Definition}[section]
\newtheorem{assumption}{Assumption}%[chapter] %
\newtheorem{proposition}{Proposition}
\newcounter{remarkcnt}
\setcounter{remarkcnt}{0}
\newenvironment{remark}
{% This is the begin code
	\stepcounter{remarkcnt} \noindent {\bf Remark \arabic{remarkcnt}.} }
%

\renewcommand{\theequation}{\arabic{equation}}
\renewcommand{\thefigure}{\arabic{figure}}
%
\newcommand{\Lower}[1]{\smash{\lower 1.5ex \hbox{#1}}}
\newcommand{\HLower}[1]{\smash{\lower .03in \hbox{#1}}}
\newcommand{\LHigher}[1]{\smash{\raise .02in \hbox{#1}}}
\newcommand{\nin}{\in \hspace*{-2.0ex}/ \hspace*{0.8ex}}
\newcommand{\x}{\bf{x}}
\newcommand{\xstar}{\bf{x^*}}
\newcommand{\STRUT}{\rule{0in}{2.5ex}}
%

\usepackage{natbib}
\bibliographystyle{chicago}
%\bibliographystyle{ormsv080}
%\bibliographystyle{plain}

% Private macros here (check that there is no clash with the style)
\usepackage[caption=false]{subfig}
%\captionsetup[subfloat]{position=top}
%\usepackage{subfig}
\captionsetup[figure]{position=t}
\captionsetup[subfigure]{position=b}
\usepackage{tablefootnote}
\usepackage{threeparttable}
\usepackage{multirow}

\usepackage{hyperref}
\hypersetup{
	colorlinks=true,
	linkcolor=blue,
	filecolor=magenta,      
	urlcolor=cyan,
}
\usepackage{filecontents}

\usepackage{booktabs}
\usepackage{graphicx}
\usepackage{xr}
\externaldocument{LSTMOpt_YilmazBuyuktahtakin2022}


\begin{document}
	\makeatletter\@input{LSTMOpt_YilmazBuyuktahtakin2022AUXfile.tex}\makeatother
	
	\renewcommand\baselinestretch{1.5}
	
	
	




%%%%%%%%%% Merge with supplemental materials %%%%%%%%%%
\pagebreak
\newpage
%\widetext
\begin{center}
\textbf{\large APPENDICES}
\end{center}
%%%%%%%%%% Merge with supplemental materials %%%%%%%%%%
%%%%%%%%%% Prefix a "S" to all equations, figures, tables and reset the counter %%%%%%%%%%
\setcounter{equation}{0}
\setcounter{figure}{0}
\setcounter{table}{0}
\setcounter{page}{1}
\setcounter{section}{0}
\makeatletter
\renewcommand{\thetable}{A\arabic{table}}
\renewcommand{\theequation}{A\arabic{equation}}
\renewcommand{\thefigure}{A\arabic{figure}}
\renewcommand{\thesection}{A\arabic{section}}
\renewcommand{\bibnumfmt}[1]{[A#1]}
\renewcommand{\citenumfont}[1]{A#1}
%%%%%%%%%% Prefix a "S" to all equations, figures, tables and reset the counter %%%%%%%%%%
\section{Results for Training LSTM Models}
\label{Results for Training LSTM Models}

For each dataset, several LSTM models are trained, and the best achieving model is selected with a process called hyperparameter tuning, as described in Section \ref{trainsection}. Table \ref{traintimes} presents the LSTM training time in CPU seconds for different datasets. The training times do not follow an identifiable pattern with $c$; however, they show an increasing trend as each of the $T$ and $f$ parameters increases. For example, the instances are solved faster when $c=8$ compared to the instances with $c=3$, but the LSTM training time is higher in three out of four datasets with $c=8$, indicating that training time is not positively correlated with the hardness of the instances for a given $T$ and $f$. The training times presented in Table \ref{traintimes} can be decreased significantly with the use of graphics processing units (GPUs). Those training times are not included in the timeML, timeimp, and timegain(\%) because the training of the models can be performed in an offline setting. However, as mentioned above, the prediction generation time using the trained LSTM model is included in the timeML, timeimp, and timegain(\%). The training times were 3.9, 4.4, and 5.2 seconds for the logistic regression and 4,430.6, 4,459.4, and 4,186.8 seconds for the random forest model. Even though they are significantly lower than the LSTM training times, their performance is inferior to the LSTM-Opt framework.

\renewcommand{\baselinestretch}{1}
\begin{table}[!htb]
\parbox{0.85\textwidth}{\caption{LSTM training times for the model with the highest validation accuracy (in CPU seconds)\label{traintimes}}}
\centering

\begin{tabular}{cccc}
%\noalign{\smallskip} \hline \noalign{\smallskip}
$f$	&	$T$	&	$c$	&	Training Time	\\	\hline
1,000	&	90	&	3	&	27,554	\\	
	&		&	5	&	19,726	\\	
	&		&	8	&	54,648	\\	\hline
10,000	&	90	&	3	&	32,086	\\	
	&		&	5	&	27,406	\\	
	&		&	8	&	70,387	\\	\hline
1,000\	&	120	&	3	&	37,794	\\	
	&		&	5	&	28,913	\\	
	&		&	8	&	72,779	\\	\hline
10,000	&	120	&	3	&	65,791	\\	
	&		&	5	&	75,147	\\	
	&		&	8	&	52,724	\\	
%\noalign{\smallskip} \hline \noalign{\smallskip}
\end{tabular}
\end{table}
\renewcommand{\baselinestretch}{}



\section{More Results on the Experiments}
\label{More Results on the Experiments}



Table \ref{t:f1,000t90} presents the results for the instances with $T = 90$ and $f = 1,000$, which are relatively easier than the instances with $T = 120$ and $f = 10,000$ in Table \ref{t:f10,000t120}. It can be seen that as the value of capacity multiplier $c$ increases from 3 to 5, the solution time decreases. As more variables are predicted, the solution time gain increases considerably with an increase in the number of infeasible instances in the test set. Predicting all binary variables (pred(\%)=100) reduces the mean solution time by more than half, but the reduction in solution time comes at a price, which is 1.45\% infeasibility in all CLSP instances and 0.13\% average optimality gap. In other words, 290 instances had infeasible predictions among 20,000 CLSP test instances, and the average objective value of the feasibly-predicted instances only deviated by 0.13\% from the average optimal objective value by CPLEX. The user cuts approach with 100\% of variables predicted achieves a time improvement of 2, with zero infeasibility and a slightly higher optimality gap. In the dataset with $c = 5$ of Table \ref{t:f1,000t90}, time improvements are similar to the previous dataset with $c = 3$, but for the same level of prediction, we observe less number of instances in the test set for which the predictions are infeasible. When $c = 8$, a low-level prediction increases the average solution time, but the complete prediction of binary variables (pred(\%)=100) achieves zero optimality gap, with only 0.01\% of the test instances having infeasible solutions, and solution time is reduced by a factor of 3. The instances presented in Table \ref{t:f1,000t90} are the easiest among all datasets. For those instances, predicting the majority of binary variables could be the most beneficial approach, reducing the solution time without a significant increase in the optimality gap or infeasibility.


\renewcommand{\baselinestretch}{1}
\begin{table}[!htb]
\caption{Summary of experiments for $f = 1,000$ and $T = 90$}
\label{t:f1,000t90}
\centering
\scalebox{0.90}{
\begin{tabular}{cccccccc}
%\noalign{\smallskip} \hline \noalign{\smallskip}
$c$     	&	       pred(\%)        	&	timeCPX	&	timeML	&	timeimp	&	timegain(\%)	&	inf(\%)	&	optgap(\%)	\\	﻿\hline
3	&	25	&	0.4	&	0.4	&	1	&	4.7	&	0.0	&	0.0	\\	
        	&	50	&		&	0.3	&	1	&	14.1	&	0.0	&	0.0	\\	
        	&	75	&		&	0.3	&	1	&	16.6	&	0.0	&	0.0	\\	
        	&	85	&		&	0.3	&	1	&	24.4	&	0.0	&	0.0	\\	
        	&	90	&		&	0.3	&	2	&	37.0	&	0.0	&	0.0	\\	
        	&	95	&		&	0.2	&	2	&	47.0	&	0.2	&	0.0	\\	
        	&	100	&		&	0.1	&	3	&	66.8	&	1.4	&	0.1	\\	
%Avg.    	&	74.3	&		&	0.3	&	1	&	30.0	&	0.2	&	0.0	\\	
        	&	       100(MS) 	&		&	0.4	&	1	&	13.0	&	0.0	&	0.0	\\	
        	&	       100(UC) 	&		&	0.3	&	2	&	37.4	&	0.0	&	0.1	\\	\hline
5	&	25	&	0.3	&	0.3	&	1	&	7.9	&	0.0	&	0.0	\\	
        	&	50	&		&	0.3	&	1	&	10.0	&	0.0	&	0.0	\\	
        	&	75	&		&	0.3	&	1	&	17.5	&	0.0	&	0.0	\\	
        	&	85	&		&	0.2	&	1	&	22.9	&	0.0	&	0.0	\\	
        	&	90	&		&	0.2	&	1	&	25.1	&	0.0	&	0.0	\\	
        	&	95	&		&	0.2	&	1	&	32.8	&	0.0	&	0.0	\\	
        	&	100	&		&	0.1	&	3	&	65.7	&	0.4	&	0.0	\\	
%Avg.    	&	74.3	&		&	0.2	&	1	&	25.9	&	0.1	&	0.0	\\	
        	&	       100(MS) 	&		&	0.4	&	1	&	-10.7	&	0.0	&	0.0	\\	
        	&	       100(UC) 	&		&	0.3	&	1	&	16.4	&	0.0	&	0.0	\\	\hline
8	&	25	&	0.3	&	0.4	&	1	&	-5.8	&	0.0	&	0.0	\\	
        	&	50	&		&	0.3	&	1	&	-5.6	&	0.0	&	0.0	\\	
        	&	75	&		&	0.3	&	1	&	0.3	&	0.0	&	0.0	\\	
        	&	85	&		&	0.3	&	1	&	6.6	&	0.0	&	0.0	\\	
        	&	90	&		&	0.3	&	1	&	14.7	&	0.0	&	0.0	\\	
        	&	95	&		&	0.3	&	1	&	20.2	&	0.0	&	0.0	\\	
        	&	100	&		&	0.1	&	3	&	70.1	&	0.0	&	0.0	\\	
%Avg.    	&	74.3	&		&	0.3	&	1	&	14.4	&	0.0	&	0.0	\\	
        	&	       100(MS) 	&		&	0.3	&	1	&	4.5	&	0.0	&	0.0	\\	
        	&	       100(UC) 	&		&	0.3	&	1	&	19.8	&	0.0	&	0.0	\\	\hline
%Table Avg.      	&	74.3	&	0.4	&	0.3	&	1	&	23.9	&	0.1	&	0.0	\\	
%Avg. (MS)       	&	       100(MS) 	&		&	0.3	&	1	&	3.1	&	0.0	&	0.0	\\	
%Avg. (UC)       	&	       100(UC) 	&		&	0.3	&	1	&	25.5	&	0.0	&	0.0	\\	\hline

%\noalign{\smallskip} \hline \noalign{\smallskip}
\end{tabular}}
\end{table}
\renewcommand{\baselinestretch}{}

Table \ref{t:f10,000t90} presents the results for instances with $T = 90$ and $f = 10,000$. These are harder than the instances shown in Table \ref{t:f1,000t90}, as seen from the mean solution time. For the instances with $c = 3$, we observe that predicting 50\% of variables reduces the average solution time by a factor of 3, with no infeasibility in the test set, and zero optimality gap. However, as more variables are predicted, solutions may become significantly infeasible. For example, at the full (100\%) prediction of the binary variables, more than half of the predictions are infeasible, which is not desired. The user cuts approach remedies this problem by resulting in all feasible solutions for all 20,000 test instances with a significant reduction in the solution time. The dataset with $c = 5$ follows a similar pattern to the dataset with $c=3$ but demonstrates less infeasibility at the higher level of predictions. Results for the dataset with $c = 8$ are similar to the instances with the same $c$ in Table \ref{t:f1,000t90}. Here, the approach that predicts the variables at higher levels achieves the most computational gain. For example, with the 75\% prediction, the solution time is improved by a factor of 2, without any loss in optimality or feasibility. It can be seen from the results that predicting variables at higher levels can be beneficial for easier instances in terms of the time gain without sacrificing feasibility or optimality.

\renewcommand{\baselinestretch}{1}
\begin{table}[!htb]
\caption{Summary of experiments for $f = 10,000$ and $T = 90$}
\label{t:f10,000t90}
\centering
\scalebox{0.90}{
\begin{tabular}{ccccccccc}
%\noalign{\smallskip} \hline \noalign{\smallskip}
$c$     	&	       pred(\%)        	&	timeCPX	&	timeML	&	timeimp	&	timegain(\%)	&	inf(\%)	&	optgap(\%)	\\	﻿\hline
3	&	25	&	3.1	&	1.9	&	2	&	38.1	&	0.0	&	0.0	\\	
        	&	50	&		&	1.1	&	3	&	63.0	&	0.0	&	0.0	\\	
        	&	75	&		&	0.4	&	8	&	87.9	&	0.4	&	0.1	\\	
        	&	85	&		&	0.3	&	12	&	91.4	&	2.0	&	0.2	\\	
        	&	90	&		&	0.2	&	14	&	92.8	&	5.3	&	0.3	\\	
        	&	95	&		&	0.2	&	15	&	93.4	&	17.5	&	0.9	\\	
        	&	100	&		&	0.1	&	22	&	95.6	&	53.9	&	1.7	\\	
%Avg.    	&	74.3	&		&	0.7	&	5	&	78.0	&	11.3	&	0.3	\\	
        	&	       100(MS) 	&		&	3.9	&	1	&	-28.2	&	0.0	&	0.0	\\	
        	&	       100(UC) 	&		&	0.3	&	10	&	90.3	&	0.0	&	1.2	\\	\hline
5	&	25	&	1.5	&	1.4	&	1	&	8.6	&	0.0	&	0.0	\\	
        	&	50	&		&	0.8	&	2	&	46.7	&	0.0	&	0.0	\\	
        	&	75	&		&	0.4	&	4	&	71.7	&	0.1	&	0.0	\\	
        	&	85	&		&	0.3	&	5	&	78.7	&	0.3	&	0.0	\\	
        	&	90	&		&	0.3	&	5	&	81.3	&	0.9	&	0.1	\\	
        	&	95	&		&	0.3	&	6	&	82.9	&	4.1	&	0.3	\\	
        	&	100	&		&	0.1	&	17	&	94.0	&	23.3	&	1.2	\\	
%Avg.    	&	74.3	&		&	0.5	&	3	&	65.1	&	4.1	&	0.2	\\	
        	&	       100(MS) 	&		&	1.5	&	1	&	5.7	&	0.0	&	0.0	\\	
        	&	       100(UC) 	&		&	0.3	&	5	&	78.4	&	0.0	&	0.7	\\	\hline
8	&	25	&	0.9	&	0.7	&	1	&	22.0	&	0.0	&	0.0	\\	
        	&	50	&		&	0.6	&	2	&	36.2	&	0.0	&	0.0	\\	
        	&	75	&		&	0.4	&	2	&	52.2	&	0.0	&	0.0	\\	
        	&	85	&		&	0.3	&	3	&	64.6	&	0.0	&	0.0	\\	
        	&	90	&		&	0.3	&	3	&	70.9	&	0.1	&	0.0	\\	
        	&	95	&		&	0.2	&	4	&	74.3	&	0.5	&	0.1	\\	
        	&	100	&		&	0.1	&	11	&	90.6	&	4.9	&	0.8	\\	
%Avg.    	&	74.3	&		&	0.4	&	2	&	58.4	&	0.8	&	0.1	\\	
        	&	       100(MS) 	&		&	0.8	&	1	&	10.8	&	0.0	&	0.0	\\	
        	&	       100(UC) 	&		&	0.3	&	3	&	67.2	&	0.0	&	0.3	\\	\hline
%Table Avg.      	&	74.3	&	1.8	&	0.5	&	3	&	70.7	&	5.4	&	0.2	\\	
%Avg. (MS)       	&	       100(MS) 	&		&	2.1	&	1	&	-12.3	&	0.0	&	0.0	\\	
%Avg. (UC)       	&	       100(UC) 	&		&	0.3	&	6	&	83.2	&	0.0	&	0.7	\\	\hline

%\noalign{\smallskip} \hline \noalign{\smallskip}
\end{tabular}}
\end{table}
\renewcommand{\baselinestretch}{}

Table \ref{t:f1,000t120} demonstrates the results for instances with $T = 120$ and $f = 1,000$, which have a similar solution time to the instances $T = 90$ and $f = 1,000$ in Table \ref{t:f1,000t90}. Also, the quality of the predictions follows a similar pattern, as in Table \ref{t:f1,000t90}. For all datasets, predictions at the lower proportions do not provide significant reductions in solution time, while predicting up to a greater extent can yield noteworthy improvement. For $c = 3$ instances, predicting 100\% of variables results in a significant solution time improvement of 4, with only 1.3\% of the instances in the test set becoming infeasible. The user cuts approach provides time improvement of 2 without causing infeasibility in any of the 20,000 test instances. For $c = 5$ instances, a significant time improvement is achieved by the full prediction of variables at the cost of 0.35\% infeasibility in the test set and 0.04\% optimality gap. For the $c = 8$ dataset, the full prediction results in a significant time improvement of 4 with a 0.02\% infeasibility and 0.01\% optimality gap. The user cuts achieve a small solution time reduction without any infeasibility in the test set.




\renewcommand{\baselinestretch}{1}
\begin{table}[!htb]
\caption{Summary of experiments for $f = 1,000$ and $T = 120$}
\label{t:f1,000t120}
\centering
\scalebox{0.90}{
\begin{tabular}{cccccccc}
%%\noalign{\smallskip} \hline \noalign{\smallskip}
$c$     	&	       pred(\%)        	&	timeCPX	&	timeML	&	timeimp	&	timegain(\%)	&	inf(\%)	&	optgap(\%)	\\	﻿\hline
3	&	25	&	0.4	&	0.4	&	1	&	13.9	&	0.0	&	0.0	\\	
        	&	50	&		&	0.4	&	1	&	16.2	&	0.0	&	0.0	\\	
        	&	75	&		&	0.4	&	1	&	16.6	&	0.0	&	0.0	\\	
        	&	85	&		&	0.3	&	2	&	36.3	&	0.0	&	0.0	\\	
        	&	90	&		&	0.3	&	2	&	40.8	&	0.0	&	0.0	\\	
        	&	95	&		&	0.2	&	2	&	49.3	&	0.2	&	0.0	\\	
        	&	100	&		&	0.1	&	4	&	73.2	&	1.3	&	0.1	\\	
%Avg.    	&	74.3	&		&	0.3	&	2	&	35.1	&	0.2	&	0.0	\\	
        	&	       100(MS) 	&		&	0.4	&	1	&	19.9	&	0.0	&	0.0	\\	
        	&	       100(UC) 	&		&	0.3	&	2	&	38.9	&	0.0	&	0.1	\\	\hline
5	&	25	&	0.3	&	0.3	&	1	&	6.4	&	0.0	&	0.0	\\	
        	&	50	&		&	0.3	&	1	&	10.9	&	0.0	&	0.0	\\	
        	&	75	&		&	0.3	&	1	&	15.0	&	0.0	&	0.0	\\	
        	&	85	&		&	0.3	&	1	&	18.3	&	0.0	&	0.0	\\	
        	&	90	&		&	0.3	&	1	&	24.9	&	0.0	&	0.0	\\	
        	&	95	&		&	0.3	&	1	&	21.1	&	0.0	&	0.0	\\	
        	&	100	&		&	0.1	&	3	&	68.4	&	0.4	&	0.0	\\	
%Avg.    	&	74.3	&		&	0.3	&	1	&	23.5	&	0.1	&	0.0	\\	
        	&	       100(MS) 	&		&	0.3	&	1	&	-3.6	&	0.0	&	0.0	\\	
        	&	       100(UC) 	&		&	0.3	&	1	&	17.4	&	0.0	&	0.0	\\	\hline
8	&	25	&	0.3	&	0.3	&	1	&	-5.4	&	0.0	&	0.0	\\	
        	&	50	&		&	0.3	&	1	&	0.2	&	0.0	&	0.0	\\	
        	&	75	&		&	0.3	&	1	&	4.7	&	0.0	&	0.0	\\	
        	&	85	&		&	0.3	&	1	&	2.1	&	0.0	&	0.0	\\	
        	&	90	&		&	0.3	&	1	&	5.5	&	0.0	&	0.0	\\	
        	&	95	&		&	0.2	&	1	&	21.8	&	0.0	&	0.0	\\	
        	&	100	&		&	0.1	&	4	&	72.2	&	0.0	&	0.0	\\	
%Avg.    	&	74.3	&		&	0.3	&	1	&	14.4	&	0.0	&	0.0	\\	
        	&	       100(MS) 	&		&	0.4	&	1	&	-17.8	&	0.0	&	0.0	\\	
        	&	       100(UC) 	&		&	0.3	&	1	&	14.8	&	0.0	&	0.0	\\	\hline
%Table Avg.      	&	74.3	&	0.4	&	0.3	&	1	&	25.6	&	0.1	&	0.0	\\	
%Avg. (MS)       	&	       100(MS) 	&		&	0.4	&	1	&	1.8	&	0.0	&	0.0	\\	
%Avg. (UC)       	&	       100(UC) 	&		&	0.3	&	1	&	25.4	&	0.0	&	0.0	\\	\hline

%%\noalign{\smallskip} \hline \noalign{\smallskip}
\end{tabular}}
\end{table}
\renewcommand{\baselinestretch}{}

\section{Predicting Instances with Different Distributions}
\label{Predicting Instances with Different Distributions}

Table \ref{gen1} presents the results on how the trained LSTM models generalize to the instances with different distributions. In the first dataset, we examine the predictive performance of the LSTM model trained on instances with $c = 3$, $f = 1,000$, and $T = 90$ on the dataset with the same $c$ and $T$, but $f = 10,000$. Here, the LSTM is trained on easier instances and used to predict the harder instances. We observe a time improvement of 2 at the 25\% prediction level, with an optimality gap under 0.5\% without any infeasibility in the test set. As the prediction level increases, time improvement increases significantly at the cost of an increased optimality gap. For example, at the 75\% prediction level, we improve the CPLEX solution time with a factor of 10 without any infeasibility but with an optimality gap of 3.8\%. In the next dataset, we examine the opposite scenario, where instances are trained on a harder dataset with $f = 10,000$ to predict easier instances with $f = 1,000$. At the lower proportions of predictions, the time improvement does not increase significantly, but predictions do also not cause any infeasible solutions. As the level of predictions increases, both the percent infeasibility in the test set and the optimality gap increase significantly. The UC remedies the infeasibility and achieves an optimality gap slightly above 5\%.

The next two datasets have completely different underlying distributions. The LSTM model is trained on easier instances with $c = 3$, $f = 1,000$ and $T = 120$ to predict harder instances with $c = 5$, $f = 10,000$ and $T = 120$. At the 25\% prediction level, a time improvement of 2 is achieved at the cost of an optimality gap, which is slightly more than 2\%, without any infeasibility in the test set. As the prediction level increases, the optimality gap increases significantly, but solutions remain highly feasible. In the opposite scenario the LSTM model is trained on instances with $c = 5$, $f = 10,000$ and $T = 120$ to predict the instances with $c = 3$, $f = 1,000$ and $T = 120$. Using an entirely different underlying distribution to make predictions leads to an increased level of infeasibility in the test set, where the prediction level of more than 75\% causes all infeasible solutions. Therefore, for those predictions, we recommend a lower-level prediction (e.g., 25\%) or the use of the CPLEX user cuts approach to remedy the infeasibility problem.

Overall, training on the easier instances to predict harder instances with a similar $c$ value can provide good results at the low level of predictions or with the UC approach. For example, the LSTM model trained with $c = 3$, $f = 1,000$, and $T = 90$ improves the CPLEX solution time with a factor of 3 without any infeasibility and with an optimality gap of 1\% at the 50\% prediction level when predicting the instances with $c = 3$, $f = 10,000$ and $T = 90$.



\renewcommand{\baselinestretch}{1}
\begin{table}[!htb]
\parbox{0.85\textwidth}{\caption{Summary of generalization experiments to test datasets with different characteristics\label{gen1}}}
\centering
\scalebox{0.75}{
\begin{tabular}{ccccccccccccc}
\multicolumn{3}{c}{LSTM Train}  					&	\multicolumn{3}{c}{Test Data}					&	       pred  	&	timeCPX	&	timeML	&	timeimp	&	timegain	&	inf	&	optgap	\\	
\cmidrule(lr){1-3}						\cmidrule(lr){4-6}																				
$c$	&	$f$	&	$T$	&	$c$	&	$f$	&	$T$	&	(\%)	&		&		&		&	(\%)	&	(\%)	&	(\%)	\\	\hline
3	&	1,000	&	90	&	3	&	10,000	&	90	&	25	&	3.1	&	1.8	&	2	&	42.6	&	0.0	&	0.3	\\	
                	&	               	&	               	&	               	&	               	&	                       	&	50	&		&	0.9	&	3	&	70.8	&	0.0	&	1.0	\\	
                	&	               	&	               	&	               	&	               	&	                       	&	75	&		&	0.3	&	10	&	89.7	&	0.0	&	3.8	\\	
                	&	               	&	               	&	               	&	               	&	                       	&	85	&		&	0.2	&	12	&	91.9	&	0.0	&	6.0	\\	
                	&	               	&	               	&	               	&	               	&	                       	&	90	&		&	0.2	&	14	&	92.9	&	0.0	&	8.0	\\	
                	&	               	&	               	&	               	&	               	&	                       	&	95	&		&	0.2	&	17	&	94.1	&	0.2	&	10.5	\\	
                	&	               	&	               	&	               	&	               	&	                       	&	100	&		&	0.1	&	30	&	96.6	&	1.1	&	13.6	\\	
%                	&	               	&	               	&	               	&	               	&	              Avg.     	&	74.3	&		&	0.5	&	6	&	82.6	&	0.2	&	6.2	\\	
                	&	               	&	               	&	               	&	               	&	                       	&	100(UC)	&		&	0.3	&	10	&	90.5	&	0.0	&	5.3	\\	\hline
3	&	10,000	&	90	&	3	&	1,000	&	90	&	25	&	0.4	&	0.4	&	1	&	5.6	&	0.0	&	0.2	\\	
                	&	               	&	               	&	               	&	               	&	                       	&	50	&		&	0.3	&	1	&	16.1	&	0.0	&	1.2	\\	
                	&	               	&	               	&	               	&	               	&	                       	&	75	&		&	0.3	&	1	&	21.2	&	0.5	&	4.7	\\	
                	&	               	&	               	&	               	&	               	&	                       	&	85	&		&	0.3	&	1	&	16.0	&	2.1	&	7.1	\\	
                	&	               	&	               	&	               	&	               	&	                       	&	90	&		&	0.3	&	1	&	21.4	&	5.6	&	9.4	\\	
                	&	               	&	               	&	               	&	               	&	                       	&	95	&		&	0.3	&	1	&	31.3	&	17.8	&	13.3	\\	
                	&	               	&	               	&	               	&	               	&	                       	&	100	&		&	0.1	&	5	&	78.7	&	54.3	&	16.4	\\	
%                	&	               	&	               	&	               	&	               	&	              Avg.     	&	74.3	&		&	0.3	&	1	&	22.6	&	11.5	&	6.5	\\	
                	&	               	&	               	&	               	&	               	&	                       	&	100(UC)	&		&	0.3	&	1	&	27.2	&	0.0	&	5.6	\\	\hline
3	&	1,000	&	120	&	5	&	10,000	&	120	&	25	&	3.0	&	1.4	&	2	&	53.9	&	0.0	&	2.1	\\	
                	&	               	&	               	&	               	&	               	&	                       	&	50	&		&	0.5	&	6	&	82.4	&	0.0	&	5.8	\\	
                	&	               	&	               	&	               	&	               	&	                       	&	75	&		&	0.2	&	12	&	91.8	&	0.0	&	22.8	\\	
                	&	               	&	               	&	               	&	               	&	                       	&	85	&		&	0.2	&	15	&	93.4	&	0.0	&	33.0	\\	
                	&	               	&	               	&	               	&	               	&	                       	&	90	&		&	0.2	&	16	&	93.7	&	0.0	&	38.7	\\	
                	&	               	&	               	&	               	&	               	&	                       	&	95	&		&	0.2	&	17	&	94.1	&	0.0	&	44.7	\\	
                	&	               	&	               	&	               	&	               	&	                       	&	100	&		&	0.1	&	28	&	96.4	&	0.0	&	51.5	\\	
%                	&	               	&	               	&	               	&	               	&	              Avg.     	&	74.3	&		&	0.4	&	7	&	86.5	&	0.0	&	28.4	\\	
                	&	               	&	               	&	               	&	               	&	                       	&	100(UC)	&		&	0.3	&	12	&	91.4	&	0.0	&	26.5	\\	\hline
5	&	10,000	&	120	&	3	&	1,000	&	120	&	25	&	0.4	&	0.4	&	1	&	5.7	&	8.6	&	1.3	\\	
                	&	               	&	               	&	               	&	               	&	                       	&	50	&		&	0.3	&	1	&	23.0	&	33.3	&	13.7	\\	
                	&	               	&	               	&	               	&	               	&	                       	&	75	&		&	0.3	&	2	&	41.5	&	81.0	&	117.8	\\	
                	&	               	&	               	&	               	&	               	&		&	85	&		&	-	&	-	&	-	&	100.0	&	-	\\	
                	&	               	&	               	&	               	&	               	&		&	90	&		&	-	&	-	&	-	&	100.0	&	-	\\	
	&		&		&		&		&		&	95	&		&	-	&	-	&	-	&	100.0	&	-	\\	
                	&	               	&	               	&	               	&	               	&		&	100	&		&	-	&	-	&	-	&	100.0	&	-	\\	
%	&		&		&		&		&	              Avg.     	&	50	&		&	0.4	&	1	&	16.1	&	74.7	&	18.5	\\	
	&		&		&		&		&	                       	&	100(UC)	&		&	0.3	&	2	&	40.4	&	0.0	&	11.8	\\	\hline
%	&		&		&		&		&	              Table Avg.       	&	71.3	&	2.1	&	0.4	&	5	&	80.0	&	21.6	&	14.3	\\	
%	&		&		&		&		&	              Avg. (UC)        	&	100(UC)	&		&	0.3	&	6	&	84.0	&	0.0	&	12.3	\\	\hline

%\multicolumn{3}{c}{LSTM Train} & \multicolumn{3}{c}{Test Data} &	soltime	&	pred(\%)	&	acc(\%)	&	F1	&	soltimeML	&	timegain(\%)	&	imp & inf(\%)	&	optgap(\%) \\
% $c$   & $f$    & $T$   &  $c$   & $f$    & $T$ &{} &{} &{} &{} &{} &{} &{} &{} \\
%%\noalign{\smallskip} \hline \noalign{\smallskip}
\end{tabular}}
\end{table}
\renewcommand{\baselinestretch}{}




%%%%%%%%%%%%%%%%%
\end{document}
%%%%%%%%%%%%%%%%%
